# Supplementary material for: Emergence of proto-organisms from bistable stochastic differentiation and adhesion
Source: arXiv:1511.02079 source file (2015-11-06)
Supplement: Supplementary file 1 [file supplementary.pdf]

# Supplementary Material
# Emergence of proto-organisms from bistable stochastic differentiation and adhesion

## I. PHYSICAL RULES OF CELL SORTING: STEINBERG'S MODEL

The model considered in this paper involves, among other components, a simple set of rules of preferential adhesion, similar to the ones used by Steinberg [1]. We will describe the simplest version of this model, made of a limited number of cell types, occupying a given two-dimensional grid. The description provides a detailed illustration of pattern-forming capacity of simple physical rules. We will also provide some examples of the specific patterns that can be created using these energy minimization rules.

The cells of this model implicitly interact through adhesion molecules. Their local displacements are driven by a tendency to minimise their interaction energy. If $M$ cell types are considered, to be indicated as $\sigma_n \in \Sigma = \{0, 1, 2, ..., M\}$, we can define the strength of the interactions among different types by means of an adhesion matrix:

$$\mathcal{J} = \begin{pmatrix} \mathcal{J}_{00} & \mathcal{J}_{01} & .... & \mathcal{J}_{0M} \\ \mathcal{J}_{10} & \mathcal{J}_{11} & .... & \mathcal{J}_{1M} \\ ... & ... & ... & ... \\ \mathcal{J}_{M0} & \mathcal{J}_{M1} & .... & \mathcal{J}_{MM} \end{pmatrix}$$

Here $J_{ab}$ is the interaction strength associated between two neighbouring cells belonging to types $a$ and $b$, respectively. For our current system we will consider three possible kinds of cells: $\sigma_0$ (grey, medium), $\sigma_1$ (white, fast growing) and $\sigma_2$ (black, waste processing). The underlying idea here is that cells will tend to attach with their neighbours with an higher probability whenever this allows the system to reach a lower energy per unit area [1]. It can be shown that

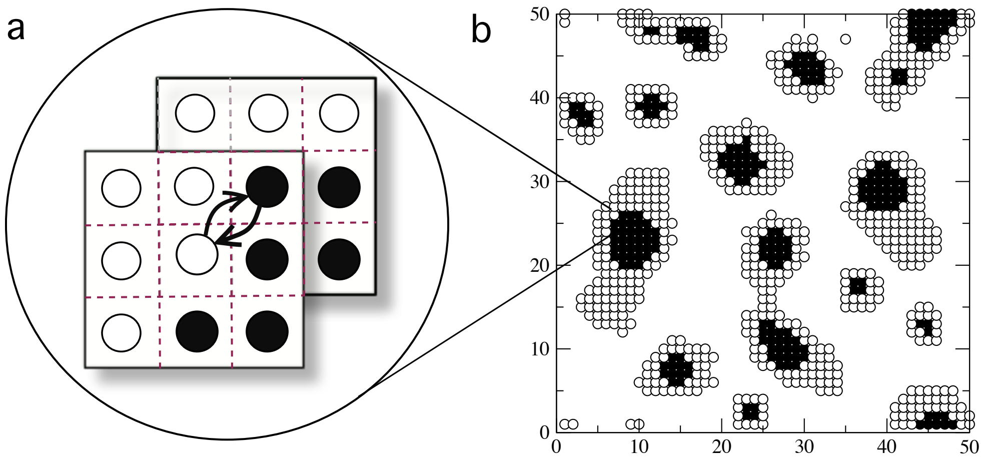


FIG. 1: Pattern formation through differential adhesion. Here the system is composed by two types of cells (open and filled circles) which are initially scattered at random on a two-dimensional lattice. Cells move and can swap their location with a neighbouring cell (a) provided that the final energy is reduced. Eventually, a stable arrangement of ordered cell assemblies (b) is obtained, in a configuration depending on the values of the adhesion matrix. In this example, the adhesion parameters satisfy $\mathcal{J}_{12} > (\mathcal{J}_{11} + \mathcal{J}_{22})/2$ and $\mathcal{J}_{11} > \mathcal{J}_{22}$.

an energy function in a given position $i, j$ can be defined as follows:

$$\mathcal{H}_{ij} = \sum_{S_{kl} \in \Gamma_{ij}} \mathcal{J}_{S_{kl}, S_{ij}} \tag{1}$$

where $\Gamma_{ij}$, in a square lattice, is the set defined by the eight nearest neighbours of a given cell in position $i, j$ (Moore's neighbourhood), each of them occupying a position $k, l$, and having a defined type $S_{kl}$.

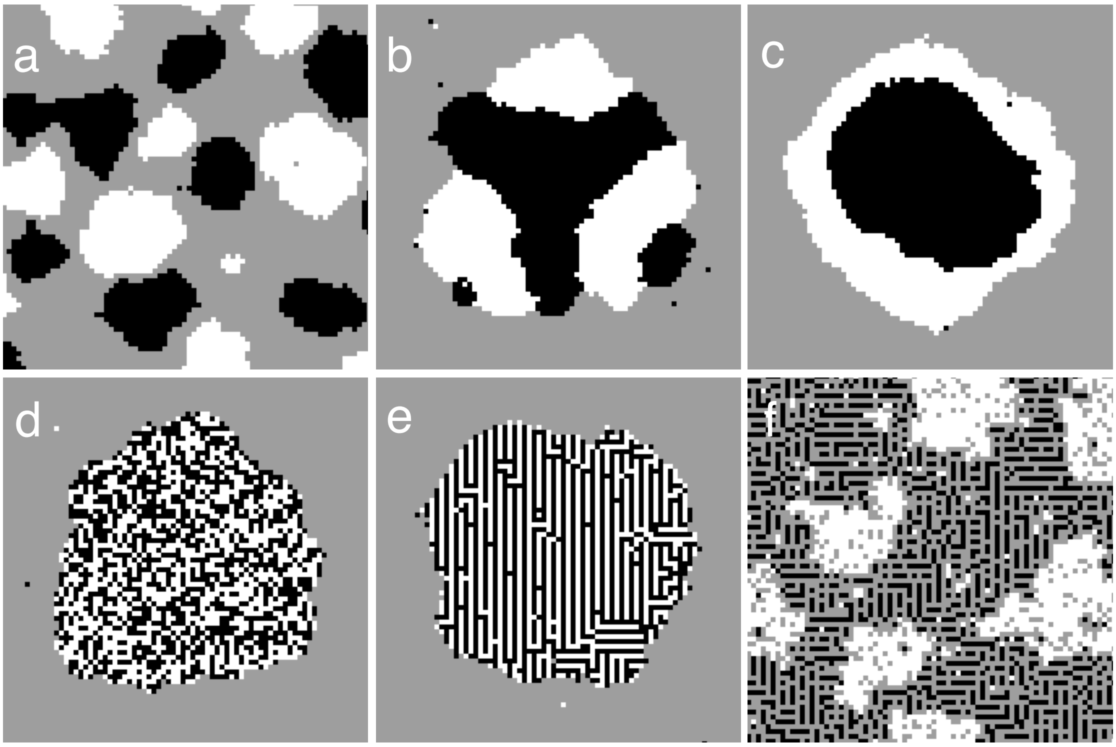


FIG. 2: Different patterns that can be observed in a cell sorting system with two cell types: separate blobs ($a$), contiguous domains ($b$), "onion" layers ($c$), random mass ($d$), labyrinth ($e$) and holed structures. Such patterns can be determinable from the adhesion matrix, and although it may take some time to reach astable configuration, these tend to form a single solid mass of cells (except for $f$-like patterns).

By evaluating this energy function we can calculate the probability that the cell in $i, j$ will move to a given neighbouring location $i', j'$, thus swapping states with that particular neighbour. In order to do this we first calculate the energy function in the case in which no swap occurs; here the energy term, named for convenience $\mathcal{H}_{ORI}$, consists of a part involving the cell in its original position and its neighbourhood set $\Gamma_{ij}$, and of a second part involving the cells' neighbour, located in $i', j'$, with its own neighbourhood $\Gamma_{i',j'}$. Then we virtually swap the positions of the cell with its neighbour in $i', j'$, and perform again the energy calculation in case of swap, $\mathcal{H}_{SWAP}$. The energy difference then, is readily defined as

$$\Delta\mathcal{H} = \mathcal{H}_{SWAP} - \mathcal{H}_{ORI} \tag{2}$$

If this difference is positive, the probability that the cell actually performs the movement will be small, whereas if it is negative it means that the system new state would have an overall lower energy, and the swap will be thus be more likely to occur. The higher the energy difference, the more accentuated the probabilities. This can be formalised by using a Boltzmann function. If we indicate as $P(S_{ij} \to S_{i'j'})$ the probability that our cell moves from $i, j$ to $i', j'$, it can be shown that

$$P(S_{ij} \to S_{i'j'}) = \frac{1}{1 + e^{\Delta\mathcal{H}/T}} \tag{3}$$

The parameter $T$ is fixed and acts as a 'temperature', essentially tuning the degree of determinism of our system. As we can see, if the energy change is positive, the so called Boltzmann factor $e^{\Delta\mathcal{H}/T}$ will be high, and the denominator

of the previous equation will be large. As a consequence, the transition probability will be small. If the difference is negative (the new state implies a reduction of energy) the Boltzmann factor will be small and the probability high: the cell displacement is likely to happen. If no difference is present, $\Delta\mathcal{H} = 0$ and the probability is 1/2 (as in a coin toss).

In figure 2*b* we display the result of a cell sorting process using $T = 10$ and a matrix favouring the attachment of cells of the same class. Specifically, we apply the following adhesion matrix:

$$\mathcal{J} = \begin{pmatrix} 0 & 0 & 0 \\ 0 & \mathcal{J}_{11} & \mathcal{J}_{12} \\ 0 & \mathcal{J}_{21} & \mathcal{J}_{22} \end{pmatrix}$$

Where $\mathcal{J}_{11} = \mathcal{J}_{22} = -20$ and $\mathcal{J}_{12} = \mathcal{J}_{21} = -10$. The result of this simulation is a well-defined pattern of spatial segregation resulting from the differential adhesion. The initial condition is a well-mixed system with equal amounts of white and black cells (type 1 and 2 respectively), and half of the sites of the lattice unoccupied (type 0). At this time there are no growth and death processes, accordingly the amount of cells of each type remains unchanged throughout the simulation.

For comparison, let us consider an opposite scenario, where cells of one type try to attach to cells belonging to the other type more than to cells of its same state. The matrix now would be $\mathcal{J}_{11} = \mathcal{J}_{22} = -10$ and $\mathcal{J}_{12} = \mathcal{J}_{21} = -20$. In this case, there is an inevitable tendency to maximise the surface among different types. The result, as shown in figure 2*e* is a labyrinth-like pattern.

As has been shown before [1,2] the final configuration of the system can be readily determined by the relations of the interaction matrix coefficients. For a system with only two cell types (1, 2) and empty medium (0), only a handful patterns are allowed, to which cell distributions converge regardless of their initial configuration on the lattice. For instance, aggregates will be formed if $2\mathcal{J}_{(1,0)} > \mathcal{J}_{(1,1)} + \mathcal{J}_{(0,0)}$ or $2\mathcal{J}_{(2,0)} > \mathcal{J}_{(2,2)} + \mathcal{J}_{(0,0)}$. Which in turn will form a single mass of cells when $2\mathcal{J}_{(1,2)} < \mathcal{J}_{(2,0)} + \mathcal{J}_{(1,0)}$. Alternatively, if these conditions are not met and cells preferentially attach to the medium, they will remain separated until -due to high density- this is no longer possible, forming the characteristic stripes shown in figure 2e.

It is worth mentioning that more sophisticated approaches were later developed by Glazier and co-workers, involving cells composed of connected lattice sites defining an embodied structure, whose shapes can change in realistic ways [3]. Having a surface enables cells to squeeze and bend, they can be stiff or engulf other cells, allowing us to incorporate a whole range of relevant biological phenomena into the model.

## II. LIST OF PARAMETERS

Here we provide the complete list of parameters used in this study, along with a short description and actual values used (or range of values for evolvable traits and phasespace variables).

Evolvable parameters were initialised to the following values: $\varepsilon_0 = 1, p_0 = 0, q_0 = 0, \mathcal{J}_{(a,b)} = 0$. Accordingly, the initial population displayed no adhesion preferences (essentially behaving as random walkers), no stochastic differentiation (since the transition rates were set to zero) and no metabolic specialisation (with $\varepsilon_0 = 1$ type 2 cells are metabolically indistinguishable from type 1 cells, i.e. they do not process $W$).

Metabolic parameters were chosen so that the relevant processes could take place, namely duplication by surpassing the appropriate $E$ threshold and death by accumulation of $W$ beyond $\Theta_{tox}$. Variations on the used values were tested and yielded similar results. Adhesion coefficient range was arbitrarily chosen and centered at zero in order to potentially display the same intensity of attractive and repulsive interactions among cells, *a priori* the most parsimonious choice.

## III. CONTINUOUS GENETIC ALGORITHM PSEUDOCODE

Listed below is the sequence of instructions, in “pseudocode”, that make up our Continuous Genetic Algorithm. As a primer for the terminology used, neighbourhood refers to a standard Moore’s neighbourhood (composed of the eight nearest lattice positions), *killing* a cell involves setting its adhesion properties to those of the empty medium, reseting its state to 0 and converting $E$ back into $N$ in that particular position. Conversely, *duplicating* a cell requires copying all parameters regarding that cell except for metabolite concentrations into the daughter cell site.

| Name | Description | Value |
|---|---|---|
| $\alpha$ | $N$ flux per time unit | [0.28 – 0.64] |
| $\beta$ | $W$ flux per time unit | [0.193 – 0.261] |
| $\gamma$ | $W$ degradation efficiency | 10 |
| $\rho$ | $N$ elaboration efficiency | 0.125 |
| $\varepsilon$ | metabolic trade-off between nutrient elaboration and waste removal | evolvable [0 – 1] |
| $\eta_N$ | $N$ decay rate | $5 \times 10^{-2}$ |
| $\eta_E$ | $E$ decay rate | $5 \times 10^{-2}$ |
| $\eta_W$ | $W$ decay rate | $5 \times 10^{-2}$ |
| $D_N$ | $N$ diffusion rate | $5 \times 10^{-2}$ |
| $D_W$ | $W$ diffusion rate | $5 \times 10^{-2}$ |
| $\xi$ | random death probability per iteration | $5 \times 10^{-4}$ |
| $\Theta_{div}$ | $E$ threshold for division | 10 |
| $\Theta_{starv}$ | $E$ threshold for death by starvation | 1 |
| $\Theta_{tox}$ | $W$ threshold for death by toxicity | 4.5 |
| $\kappa$ | scaling factor between genetic and adhesion processes | $10^{-3}$ |
| $p$ | transition probability from type 1 to type 2 cells | evolvable [0 – 1] |
| $q$ | transition probability from type 2 to type 1 cells | evolvable [0 – 1] |
| $\mathcal{J}_{(a,b)}$ | interaction coefficient between cells of type a & b | evolvable [-50 – 50] |
| $T$ | temperature used to validate cell swap in the movement step using the Boltzmann distribution | 10 |
| $\mu$ | mutation rate per "gene" and division | $5 \times 10^{-3}$ |
| $dt$ | time interval per algorithm iteration (used in the *Euler* numerical integration) | $10^{-1}$ |

TABLE I: List of parameter values used in the article and description of their role in the model. Separated by lines are the parameters corresponding to each of the main areas of the model, namely: metabolism, genetics, cell sorting and general aspects of the simulation, respectively from top to bottom.

```
initialize lattice and variables
create initial population of cells

loop for target iterations
    for all non-empty sites (x, y) in the lattice Ω do
        choose random neighbour (x', y')
        compute energy in the current cellular arrangement
        compute energy if sites (x, y) and (x', y') were swapped
        if energy difference is negative then
            switch states, genotypes and metabolite concentrations between sites (x, y) and (x', y')
        else
            draw a random number π from a uniform distribution [0,1)
            if π is smaller than the probability following the Boltzmann distribution then
                switch states, genotypes and metabolite concentrations between sites (x, y) and (x', y')
            end if
        end if
    end for

    for all sites in the lattice Ω do
        if cell state is empty then
            calculate addition of N, W
            calculate diffusion of N, W and decay of N, W, E
        else
            calculate diffusion of N, W and decay of N, W, E

            draw a random number π from a uniform distribution [0,1)
            if W ≥ Θ_tox OR E ≤ Θ_starv OR π ≤ ξ then
                kill cell
            else

                draw a random number π from a uniform distribution [0,1)
                if π ≤ κp AND current type is 1 then
                    set type to 2
                else
                    draw a random number π from a uniform distribution [0,1)
                    if π ≤ κq AND current type is 2 then
                        set type to 1
                    end if
                end if

                if E ≥ Θ_div AND there are empty sites in the neighbourhood then
                    duplicate cell and split resources
                    for all genotypic traits do
                        draw a random number π from a uniform distribution [0,1)
                        if π ≤ μ then
                            mutate trait in the new cell
                        end if
                    end for
                end if
            end if
        end if
    end for

    for all sites in the lattice Ω do
        update N, E and W values
    end for
end loop
```

Diffused quantities were computed using the standard discretisation for a lattice:

$$D_\nu \bigtriangledown^2 \nu_{x,y} = D_\nu \sum_{(x',y')\in\Gamma_{x,y}} [\nu_{x',y'} - \nu_{x,y}],$$

where $\nu$ is a placeholder for the diffusing substances ($N$ and $W$) and $\Gamma_{x,y}$ is the Moore's neighbourhood (of size 1) centered on the site $(x, y)$.

## IV. MEASURES OF SPATIAL AND GENOMIC COMPLEXITY

### A. Variance

Genetic diversity of an ensemble of cells living at a particular time point was calculated using:

$$\sigma^2(G) = \frac{1}{n}\sum_{j=1}^{L}\sum_{i=1}^{n}[g_j^i - \mu_j]^2,$$

where $G$ stands for the complete genotype of a population, composed of $n$ cells each having $L$ independent traits. A particular trait in the genotype of the *ith* cell is then denoted as $g_j^i$, and its average value in the population $\mu_j$. Prior to the variance calculation, the adhesion coefficients of cells were normalized to the same range as the *Stochastic Phenotypic Switching* and the *Metabolic trade-off* $\varepsilon$ parameters ($[0-1]$). Given that the adhesion coefficient values range from -50 to +50 the following simple linear transformation was applied:

$$g_j^{norm} = \frac{g_j^{adh} + 50}{100}.$$

This ensures that all cellular traits have potentially the same impact on genetic diversity and the values obtained from this measure are not mainly governed by a subset that happen to have larger ranges.

Also, variance data shown in the main text is "total variance", not an average per *locus.* That is, variance obtained with this method is normalised to population size at that time step but is not normalised to genotype size $L$, showing then the accumulated variance across "genes".

### B. Mutual information

In the main text we use a modified version of Mutual Information as a way to characterise spatial order or complexity. Normally, this measure is simply used to characterise the mutual dependence of two variables [4], and given two discrete random variables $x, y$ it can be defined as:

$$I(X;Y) = \sum_{x\in X}\sum_{y\in Y} p(y)p(x|y)\log_2(\frac{p(x|y)}{p(x)}) \tag{4}$$

where  and $Y$ represent the set of discrete states that the two variables $x$ and $y$ can take. The marginal probabilities $p(x)$ and $p(y)$ represent the probability that the two variables $x$ and $y$ are found in a given state of the set $X$ or $Y$ respectively. The conditional probability $p(x|y)$ measures the probability to find $x$ in a given state when variable $y$ is fixed to a specific state.

If we want to measure the mutual information between the $n$ possible states of the set of states $m$ that a cellular automata in a 2D lattice can take, we can adapt this definition to:

$$I(S_{ij}; S_{kl} \in \Gamma_{ij}^{\lambda}) = \sum_{S_{ij}\in n}\sum_{S_{kl}\in m} p(S_{ij})p(S_{kl}|S_{ij})\log\frac{p(S_{kl}|S_{ij})}{p(S_{kl})} \tag{5}$$

where $S_{ij}$ is the state of a cellular automata occupying a defined position $i, j$ in the lattice, and $S_{kl} \in \Gamma_{ij}^{\lambda}$ represent the ensemble of nearest neighbors of a given position $i, j$ up to a given distance $\lambda$ in lattice sites (Moore's neighborhood of size $\lambda$), each of them occupying a position $k, l$, and having a defined state $S_{kl}$. So, for instance, $p(S_{ij} = n_1)$ represents the probability to find the cellular automata in the $n_1$ state, and is simply given by

$$p(S_{ij} = n_1) = \frac{\sum_{i,j}\delta_{(n_1, S_{ij})}}{A}, \tag{6}$$

where we make use of Kronecker's delta function $\delta_{(n_1,S_{ij})}$, which equals 1 in the case that $S_{ij} = n_1$, and 0 otherwise). The value $A$ is the area of the 2D lattice. As for $p(S_{kl} = n_1)$, theorically this would represent the probability that, travelling through all the positions $i, j$ of the lattice - independently from their state - one randomly chosen neighbour $S_{kl} \in \Gamma_{ij}^{\lambda}$ of a given position $i, j$ has state $n_1$. This coincides with the probability to find the cellular automata in the $n_1$ state all over the lattice, so that the probability is again given by

$$p(S_{kl} = n_1) = \frac{\sum_{k,l} \delta_{(n_1,S_{kl})}}{A} \tag{7}$$

Finally, $p(S_{kl} = n_2 | S_{ij} = n_1)$ represents the probability that, for a given state $S_{ij} = n_1$, one of its neigbours $S_{kl} \in \Gamma_{ij}^{\lambda}$ will have the state $n_2$. Here the two values $n_1$ and $n_2$ represent any possible combination of the set of states $m$, i.e. they may or may not coincide.

Note that in our case $S_{ij}$ and $S_{kl}$ can take the discrete values 0 , 1 and 2, representing respectively the medium and the two possible states of the living cells. We observed that in our model a Moore's neighborhood with $\lambda = 1$) it is not optimal to assess the mutual information between two variables, therefore we chose to extend neighborhood at $\lambda = 3$.

Following this definition, the spatially constrained information will be higher when the cellular states contain information about each other at the specified distance or less. Conversely, if the spatial distribution of cells is random, their mutual information will tend to zero. It is important to stress that, as indicated in Eq.2, the total mutual information is given by the sum on mutual information between all the pairs of possible discrete states that we can find in our system.

## V. GENOTYPE ISOSURFACE

Figure 3 of the main text portrays the evolutionary process as gene frequencies change in multiple, distinct populations. This can be readily visualised by the movement of genotype distributions in the $x$ and $y$ axes, yet at some time steps the dot density is too big to accurately represent population levels. In order to easily capture these shifts an envelope surrounding the individual dots is displayed. This objects defines an arbitrary boundary in population density, showing in the time dimension and also in genotype space where the center of mass of population genotypes lies.

In order to create the envelope, a standard *marching cubes* [5] algorithm was used. Firstly, the space defined by the genotype and time was regularly discretized. Each position of this 3D lattice was assigned a value proportional to the number of individuals (dots) inside its boundaries. This density dependent object was smoothed following the criteria described in [5]. The isosurface was then calculated using an arbitrarily chosen density threshold, and is shown to closely match and surround the discrete species observed directly and with other analytic methods (see next section).

## VI. SNAPSHOTS OF THE GENOTYPE SPACE

The representation of the evolutionary process shown in Figure 3 of the main text enables the straightforward visualization of the continuity of genotypes, that is, that every cell and every species comes from an entity of the same category that is closely located in the genotype space. Nonetheless, it hampers the interpretation of where do the species exactly lie in the $\Phi$ and $\Psi$ axes. Supplementary figure 1 shows temporal snapshots of population density in the same genotype space used in the main text, albeit all shown plots share the same range and mark the axes center with white lines in order to ease interpretation.

The first thing to notice is how similar is the first snapshot of the three scenarios, yet some modifications seem to have already happened, forecasting the outcome of the evolutionary process. Namely, in $b$ we can observe how the U1 population is mostly located at $\Psi \leq 0$ (meaning that even if there are no type 2 cells to) evaluate this adhesion property, cells are exploring an essentially neutral landscape. As help for interpretation we also offer a guide for what each quadrant of $\Phi, \Psi$ space stand for in supplementary figure 2.

It is also worth noting that although mutation introduces a bell shaped distribution into the "master genotype", accepted variance into the genotype is different depending on the cellular function. For instance, in the later stages of case $a$ we observe that the genotype distribution in $\Phi$ space is thinly confined around an optimum value. Conversely, in the unicellular lineages of both scenario $a$ and $b$ a much broader shape is observed, suggesting that the selective pressures in each case are completely different.

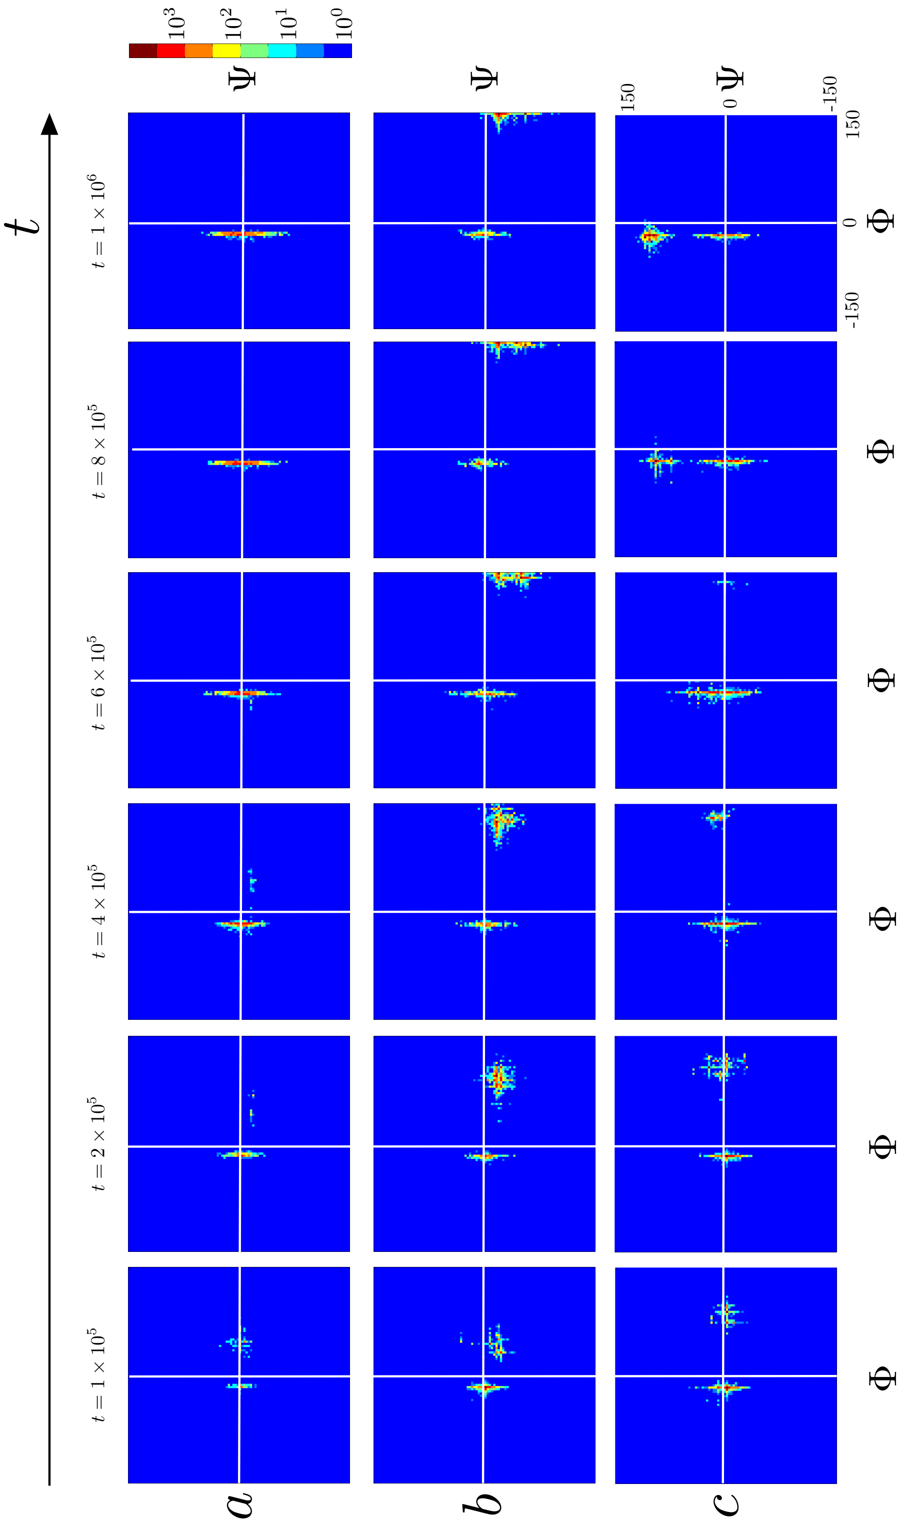


FIG. 3: Sequential snapshots of population density in genotype space using heat maps. Here we show, for each of the three filogenies of the main text ($a, b$ and $c$), a series of population density maps in logarithmic scale at time steps 1, 2, 4, 6, 8 and 10×$10^5$ iterations. All plots display discretized genotypes (100 × 100 lattice) and share the same axes limits: $\Phi = 2\mathcal{J}_{(1,0)} - \mathcal{J}_{(1,1)}$ =[-150 – 150], $\Psi = 2\mathcal{J}_{(2,0)} - \mathcal{J}_{(2,2)}$ =[-150 – 150]. Population value, as number of cells displaying a particular genotype, is represented using the colour code displayed on the right side of the figure, following a logarithmic scale.

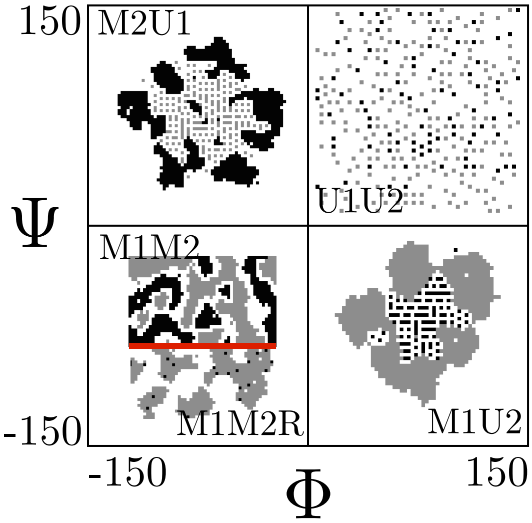


FIG. 4: Main genotypes observed in the genetic algorithm and their position in genotype space. Given the discrete nature of the cell sorting algorithm, each quadrant in this $\Phi, \Psi$ space can be readily assigned a phenotype, and all positions in the quadrant should qualitatively display the same structures. Further evolution into extreme values is still observed in all three presented scenarios, seemingly caused by competition among cells for resources.

## VII. PRINCIPAL COMPONENT ANALYSIS

Figure 3 (main text) shows the speciation process with the divergence of a single, continuous population in genotype space into discrete or discontinuous populations. Only three dimensions of the cell genotype are used (i.e., the capacity to create homo-aggregates $\Phi, \Psi$ and the waste management capabilities $\varepsilon$). At this descriptive level, some species are shown to be heterogeneous (mainly in terms of $\varepsilon$) and, perhaps, could still be further separated into smaller populations using the rest of traits. To discriminate subpopulations inside the already defined species we performed a Principal Component Analysis using Matlab 2013b package (*pca* function, dimensions normalised following the procedure described in section **III.A**, the three datasets were analysed separately). Supplementary Figure 3 shows, for the three scenarios described in the main text, the genotypes of living individuals at $t = 8 \times 10^5$ in the newly defined axes (first and second principal components).

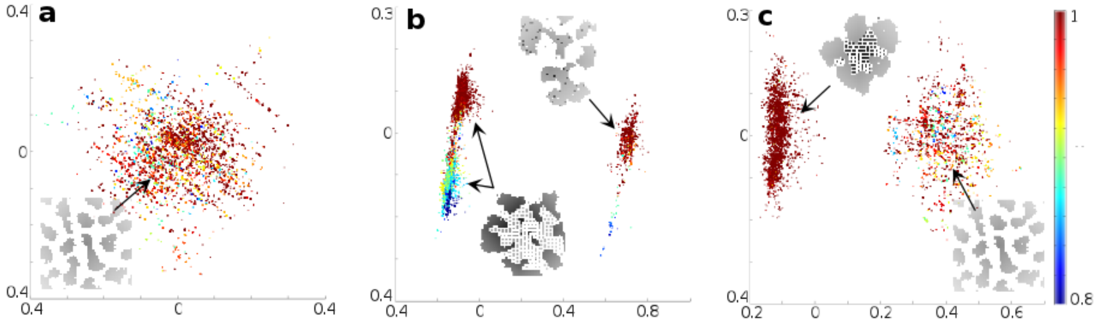


FIG. 5: Principal component analysis of the population genotype. Consistently with our analysis, the same discrete populations appear. Here as a guide to the eye we have depicted $\varepsilon$ for each individual using a colour scale (same range for all plots [0.8, 1]) as well as the expected phenotype simulated in isolation. The two first components explained 61.06%, 93.72% and 89.72% of the variability in the data respectively.

As it can be observed, no new lineages (separate dot distributions) appear using this analysis beyond the already described. This consolidates the treatment shown in the main text, which offers at the same time a clear connection to the physical processes happening in the simulation, since the axis are meant to display actual features and not to accumulate the maximum variability. However, some populations are better separated using this procedure (M2U1 and M2U1 with lower $\varepsilon$), potentially leading us to consider them different species.

## VIII. EVOLUTIONARY AND SHORT SCALE DYNAMICS

Four movies are included to better demonstrate the processes at work in our model. All four display the state $\{0, 1, 2\}$ of each element of the lattice (size $400 \times 400$) using the same colour code established before. The first one (SM1), corresponds to a simulation with the parameter set $\alpha = 0.56, \beta = 0.247$; and displays the fine grained phenomena described in main text (each frame corresponds to 250 iterations of our algorithm). Particularly:

- Cyclic breakage and duplication of the outer layer.
- Regeneration of the external layer by the inner clusters.
- Regrowth of the whole pattern by a isolated group of type 1 cells previously forming an internal cluster.

The following three are meant to help the reader visualise the evolutionary processes (each frame corresponds to 5000 iterations) and display, for each of the three cases shown in Figure 3 of the main text, the corresponding evolution of cellular states. In particular, it is worth to notice the oscillatory dynamics appearing in the second scenario (SM3) and the evolution of new strains and the scales involved in population substitution (SM4).

## IX. REFERENCES

[1] - Steinberg, M S. 1975. Adhesion-Guided Multicellular Assembly: A Commentary upon the Postulates, Real and Imagined, of the Differential Adhesion hypothesis, with Special Attention to Computer Simulations of Cell Sorting. J. Theor. Biol. 55 (2):431-43.

[2] - Goel, N, R D Campbell, R Gordon, R Rosen, H Martinez, and M Ycas. 1970. Self-Sorting of Isotropic Cells. J. Theor. Biol. 28 (3): 423-68.

[3] - Glazier, J. A. and Graner, F. 1993. Simulation of the differential adhesion driven rearrangement of biological cells. Emergence of multicellularity in a model of cell growth, death and aggregation. Phys. Rev. E 47: 2128-2154

[4] - Cover, T. M., and Thomas, J. A. (2012). Elements of information theory. John Wiley & Sons.

[5] - Lorensen, W. E. and Cline, H. E. (1987). Marching cubes: A high resolution 3d surface construction algorithm. ACM Computer Graphics 21 (4): 163-169.

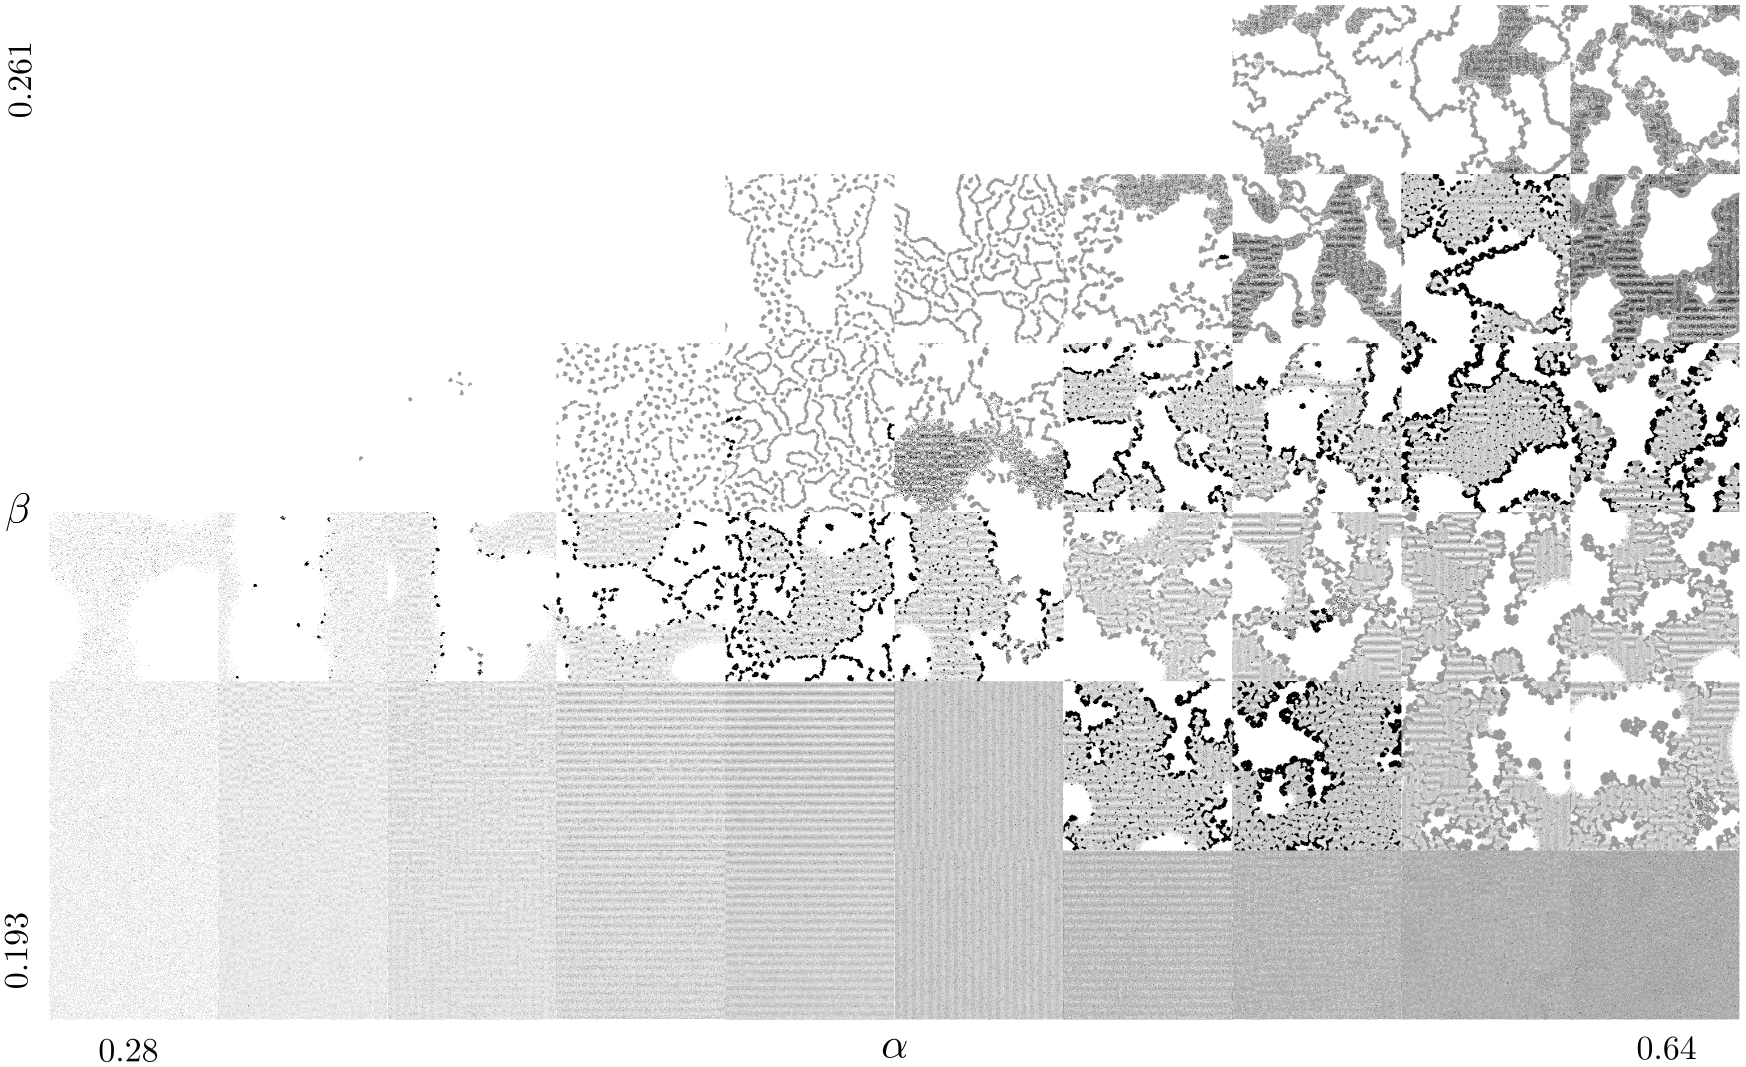


FIG. 6: The complete phasespace. For the same range of $\alpha$ and $\beta$ values used in the main text, we show the full simulation space ($400 \times 400$ square lattice) instead of a representative region at $5 \times 10^5$ algorithm iterations. Nested structures and complex organizations are pervasive throughout the multicellular region of the phasespace. Some islands of living type 1 cells can be found across the high $W$ boundary which are not displayed in the main text.
